# Supplementary material for: Active wave-particle clusters
Source: arXiv:2503.07201 ancillary file (2025-11-03)
Supplement: Supplementary file 1 [file Supplemental_Material_HNA.pdf]

# Supplemental Material for “Hydrodynamic nuclear analogs with active wave-particle clusters”

Rahil N. Valani<sup>1\*</sup> and David M. Paganin<sup>2</sup>

<sup>1</sup>*Rudolf Peierls Centre for Theoretical Physics, Parks Road,  
University of Oxford, OX1 3PU, United Kingdom and*

<sup>2</sup>*School of Physics and Astronomy, Monash University, Victoria 3800, Australia*

This Supplemental Material accompanies our Letter titled “Hydrodynamic nuclear analogs with active wave-particle clusters”. It is structured as follows. Section I explains how to proceed from the dimensional to the dimensionless forms of the key integrodifferential equation given in Eqs. (1) and (2) of the main text. We then explain the means by which we numerically solve this governing equation, in Sec. II. Section III presents results on static configurations of active wave-particle clusters at low memory. Chaotic collective excitations and diffusive cluster motion are treated in Sec. IV. Next, Sec. V discusses the convolution approximation that may be used to estimate the bag-like time-averaged wave field associated with an active wave-particle cluster. Section VI studies two different classes of behavior associated with

particles that are ejected from a wave-particle cluster, namely (i) ejected particles that completely escape the cluster and (ii) ejected particles that are confined to an annular “halo” region in the vicinity of the main cluster. Finally, Sec. VII discusses additional avenues for future research and possible broader implications of our work, beyond what is already outlined in the main text.

## I. NON-DIMENSIONALIZATION OF THE INTEGRODIFFERENTIAL EQUATION OF MOTION

The dimensional form of the integrodifferential equation for the motion of a single wave-particle entity (WPE) in two horizontal dimensions is given by [1]

$$m\ddot{\mathbf{x}}_p + D\dot{\mathbf{x}}_p = -\frac{mgAk_F}{T_F} \int_{-\infty}^t W'(k_F|\mathbf{x}_p(t) - \mathbf{x}_p(s)|) \frac{\mathbf{x}_p(t) - \mathbf{x}_p(s)}{|\mathbf{x}_p(t) - \mathbf{x}_p(s)|} e^{-\frac{(t-s)}{T_F \text{Me}}} ds. \quad (1)$$

Here,  $m$  is the droplet mass,

$$k_F = 2\pi/\lambda_F \quad (2)$$

is the Faraday wavenumber corresponding to the Faraday wavelength  $\lambda_F$  (i.e. the wavelength of the droplet-generated waves),  $g$  is the gravitational acceleration,  $A$  is the amplitude of the surface waves,  $\text{Me}$  is the memory parameter that prescribes the decay rate of droplet-generated waves and  $T_F$  is the Faraday period (i.e. the period of the droplet-generated standing waves). See Oza *et al.* [1] for more details and explicit expressions for these parameters.

We start by non-dimensionalizing Eq. (1) using

$$\mathbf{x}' = k_F \mathbf{x} \quad (3)$$

and

$$t' = Dt/m. \quad (4)$$

Dropping primes on the dimensionless variables gives

$$\ddot{\mathbf{x}}_p + \dot{\mathbf{x}}_p = -R \int_{-\infty}^t W'(|\mathbf{x}_p(t) - \mathbf{x}_p(s)|) \frac{\mathbf{x}_p(t) - \mathbf{x}_p(s)}{|\mathbf{x}_p(t) - \mathbf{x}_p(s)|} e^{-\frac{(t-s)}{\tau}} ds,$$

where we have introduced the dimensionless wave amplitude

$$R = m^3 g A k_F^2 / (D^3 T_F) \quad (5)$$

and the dimensionless memory time

$$\tau = DT_F \text{Me} / m. \quad (6)$$

If we now consider many interacting WPEs and also include a short-range repulsive force to take into account the finite particle size, then we recover the dimensionless equations in Eqs. (1) and (2) of the main text.

## II. NUMERICAL IMPLEMENTATION DETAILS

We solve the integrodifferential trajectory equations in Eqs. (1) and (2) of the main text using a modified

\* rahil.valani@physics.ox.ac.uk

Euler method. For  $t < 0$ , the WPEs are assumed to be stationary. The particle positions

$$\mathbf{x} = (x_p, y_p) \quad (7)$$

for  $N$  WPEs are initialized randomly in a circle of radius  $a\sqrt{N/2}$ , while making sure that they are not overlapping. The new position of the  $i$ th particle is calculated from the

old position using a forward Euler step

$$\begin{aligned} x_{pi}(t_{n+1}) &= x_{pi}(t_n) + \Delta t u_{pi}(t_n) \\ y_{pi}(t_{n+1}) &= y_{pi}(t_n) + \Delta t v_{pi}(t_n), \end{aligned}$$

where

$$\dot{\mathbf{x}} = (u_{pi}, v_{pi}) \quad (8)$$

is the particle velocity. To calculate the new velocity, we use the updated position and a backward Euler step via

$$\begin{aligned} u_{pi}(t_{n+1}) &= u_{pi}(t_n) + \Delta t \left[ -u_{pi}(t_{n+1}) - R \int_0^{t_n} W'(|\mathbf{x}_{pi}(t_{n+1}) - \mathbf{x}_{pi}(s)|) \frac{x_{pi}(t_{n+1}) - x_{pi}(s)}{|\mathbf{x}_{pi}(t_{n+1}) - \mathbf{x}_{pi}(s)|} e^{-(t_{n+1}-s)/\tau} ds \right. \\ &\quad \left. - R \sum_{\substack{j=1 \\ j \neq i}}^N \int_0^{t_n} W'(|\mathbf{x}_{pi}(t_{n+1}) - \mathbf{x}_{pj}(s)|) \frac{x_{pi}(t_{n+1}) - x_{pj}(s)}{|\mathbf{x}_{pi}(t_{n+1}) - \mathbf{x}_{pj}(s)|} e^{-(t_{n+1}-s)/\tau} + \sum_{\substack{j=1 \\ j \neq i}}^N F_{xij}^{rep} \right] \end{aligned} \quad (9)$$

$$\begin{aligned} v_{pi}(t_{n+1}) &= v_{pi}(t_n) + \Delta t \left[ -v_{pi}(t_{n+1}) - R \int_0^{t_n} W'(|\mathbf{x}_{pi}(t_{n+1}) - \mathbf{x}_{pi}(s)|) \frac{y_{pi}(t_{n+1}) - y_{pi}(s)}{|\mathbf{x}_{pi}(t_{n+1}) - \mathbf{x}_{pi}(s)|} e^{-(t_{n+1}-s)/\tau} ds \right. \\ &\quad \left. - R \sum_{\substack{j=1 \\ j \neq i}}^N \int_0^{t_n} W'(|\mathbf{x}_{pi}(t_{n+1}) - \mathbf{x}_{pj}(s)|) \frac{y_{pi}(t_{n+1}) - y_{pj}(s)}{|\mathbf{x}_{pi}(t_{n+1}) - \mathbf{x}_{pj}(s)|} e^{-(t_{n+1}-s)/\tau} + \sum_{\substack{j=1 \\ j \neq i}}^N F_{yij}^{rep} \right], \end{aligned} \quad (10)$$

where

$$\begin{aligned} F_{xij}^{rep} &= \begin{cases} K \frac{x_{pi}(t_{n+1}) - x_{pj}(t_{n+1})}{|\mathbf{x}_{pi}(t_{n+1}) - \mathbf{x}_{pj}(t_{n+1})|} (a - |\mathbf{x}_{pi}(t_{n+1}) - \mathbf{x}_{pj}(t_{n+1})|), & \text{if } |\mathbf{x}_{pi}(t_{n+1}) - \mathbf{x}_{pj}(t_{n+1})| < a \\ 0, & \text{otherwise} \end{cases} \\ F_{yij}^{rep} &= \begin{cases} K \frac{y_{pi}(t_{n+1}) - y_{pj}(t_{n+1})}{|\mathbf{x}_{pi}(t_{n+1}) - \mathbf{x}_{pj}(t_{n+1})|} (a - |\mathbf{x}_{pi}(t_{n+1}) - \mathbf{x}_{pj}(t_{n+1})|), & \text{if } |\mathbf{x}_{pi}(t_{n+1}) - \mathbf{x}_{pj}(t_{n+1})| < a \\ 0, & \text{otherwise.} \end{cases} \end{aligned}$$

The integrals in Eqs. (9) and (10) were performed using the trapezoidal rule, where we consider the contribution from all the previous impacts for the first 1280 timesteps relative to memory ( $t/\tau = 20$ ) and then the contribution from the last 1280 impacts for  $t/\tau > 20$ . At 1280 previous impacts, the exponential damping factor has reached  $e^{-20} \approx 10^{-9}$  so we neglect all contributions from impacts beyond 1280 previous steps.

### III. STATIC CONFIGURATION AT LOW-MEMORY

At very small values of the memory parameter  $\tau$ , we obtain a static configuration of the cluster where the arrangement of the particles depends on the particle size  $a$ , the number of particles in the cluster  $N$  and (weakly) on

the memory parameter  $\tau$ . A comparison of two different static particle arrangements in a cluster of 10 particles of two different sizes  $a = 1.01$  and  $a = 1.63$  is shown in Fig. 1. In experiments with superwalking droplets, a tightly bound crystalline lattice arrangement of particles has been observed at low memory [2].

### IV. CHAOTIC COLLECTIVE EXCITATIONS AND DIFFUSIVE CLUSTER MOTION

In addition to the well-defined collective modes of excitation presented in the main text of this Letter, one usually finds chaotic collective excitations at memory values that are intermediate between those associated with the different distinct modes. For active wave-particle clusters with small particles of size  $a = 1.01$ , an example is

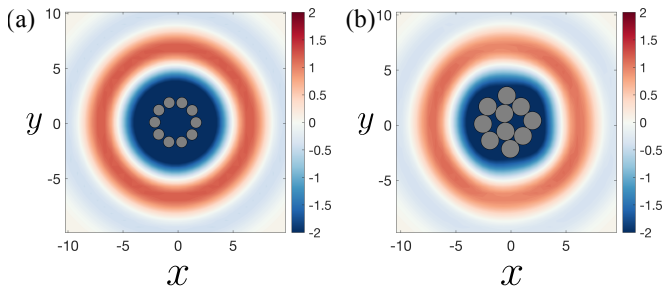

FIG. 1. Static configurations of active wave-particle clusters at low memory. A cluster of 10 WPEs self-organize into a static configuration based on the size of each particle, as shown in panels (a) and (b) for particle sizes  $a = 1.01$  and  $a = 1.63$ , respectively. Other parameters were fixed to  $R = 0.77$ ,  $\alpha = 0.16$ ,  $\tau = 0.30$  for panel (a), and  $R = 1.72$ ,  $\alpha = 0.16$ ,  $\tau = 0.56$  for panel (b).

shown in Fig. 2 and Supplemental Video S7. This corresponds to a value for the memory that is intermediate between values associated with breathing and crushing modes. In addition to aperiodic oscillations, the center of mass (COM) of the cluster jitters around showing diffusive motion (see Fig. 2(c)), analogous to a dense suspension of active particles confined in a droplet [3].

For an active wave-particle cluster of particles of size  $a = 1.63$ , one observes that for values of the memory parameter  $\tau$  just below the onset of a rotating mode, a chaotic intermittent rotating mode is observed. As shown in Fig. 3 and Supplemental Video S8, the cluster intermittently switches between clockwise and counterclockwise rotation.

## V. APPROXIMATING THE TIME-AVERAGED WAVE FIELD AS A CONVOLUTION

Durey *et al.* [4] showed that if the chaotic dynamics of the WPE is ergodic and a stationary probability distribution exists, then the mean wave-field  $\bar{W}(\mathbf{x})$  can be obtained by the convolution integral

$$\bar{W}(\mathbf{x}) = \int_{\mathbb{R}^2} W_B(\mathbf{x} - \mathbf{y}) \mu(\mathbf{y}) d\mathbf{y}, \quad (11)$$

where  $W_B(\mathbf{x})$  is the wave field of a stationary WPE, i.e. the wave field from infinitely many bounces at the origin, and  $\mu(\mathbf{x})$  is the stationary probability distribution of the particle. The wave field of a stationary WPE is given by

$$\begin{aligned} W_B(\mathbf{x}) &= R \int_{-\infty}^t \cos(|\mathbf{x}|) e^{-\alpha^2 |\mathbf{x}|^2} e^{-(t-s)/\tau} ds, \\ &= R \tau \cos(|\mathbf{x}|) e^{-\alpha^2 |\mathbf{x}|^2}. \end{aligned}$$

Although the assumption of ergodicity may not always be satisfied for chaotic dynamics, it is natural to study the consequence of the simplifying assumption that a WPE

*uniformly* explores the space within the cluster, i.e. that  $\mu(\mathbf{x})$  has a uniform distribution inside a circle of radius equal to the mean cluster radius. A comparison of the mean wave field from a numerical simulation with the above convolution approach is shown in Fig. 4, for the system studied in our Letter. We can see that the convolution calculation approximately captures both the qualitative and the quantitative features of the bag-like mean wave field of the active wave-particle cluster.

## VI. ESCAPE AND BOUNDED PARTICLES AFTER DECAY

For active wave-particle clusters that result in particle ejection at large values of the memory parameter  $\tau$ , we find that the ejected particle can have two different fates depending on the spatial extent of the particle-generated waves. As shown in Fig. 5 and Supplemental Video S9, if the spatial extent of the particle-generated waves is large (i.e.  $\alpha$  is small), after ejection the particle stays bound to the cluster but cannot penetrate back inside the cluster due to the wave barrier. Hence, the particle orbits the cluster. This is analogous to a halo nucleus wherein a core nucleus is surrounded by one or more orbiting protons or neutrons [5]. In the second scenario, as shown in Fig. 6, if the spatial extent of the particle-generated waves is small (i.e.  $\alpha$  is large), after ejection the particle can completely escape the cluster.

## VII. FUTURE WORK AND DISCUSSION

To augment what is given in the main text of the Letter, we here list several possible avenues for future work:

1. It would be useful to investigate whether there exists an active-particle-cluster analog of the *semi-empirical mass formula* of nuclear physics [6]. Such a formula might look something like

$$B \approx aN - b\sqrt{N} + \dots, \quad (12)$$

where  $B$  is the binding energy of an active-particle cluster,  $aN$  is a bulk term proportional to the number of particles  $N$  in the cluster (with  $a > 0$ ),  $-b\sqrt{N}$  is a surface term proportional to the number of particles along the perimeter of the cluster (with  $b > 0$ ), and additional terms may be employed to model effects such as particle-particle repulsion. Perhaps such a formula could be used to determine a condition for an active-particle cluster to be stable.

2. We only considered one type of active particle, in modeling active-particle clusters. However, the governing system of equations [Eqs. (1) and (2) in the main text] could be easily generalized to two or more active-particle types. In particular, if *two*

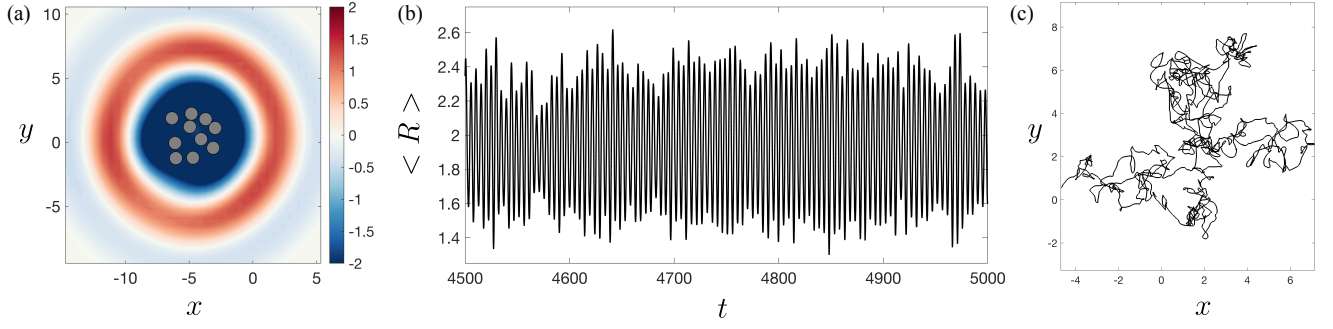

FIG. 2. Chaotic breathing mode of an active wave-particle cluster. (a) Snapshot of a cluster of 10 particles each of size  $a = 1.01$  exhibit a chaotic breathing mode for  $R = 0.77$  and  $\tau = 0.93$  (see also Supplemental Video S7). (b) Time series of mean radius of the cluster showing aperiodic oscillations and (c) trajectory of the center of mass (COM) of the cluster showing diffusive motion.

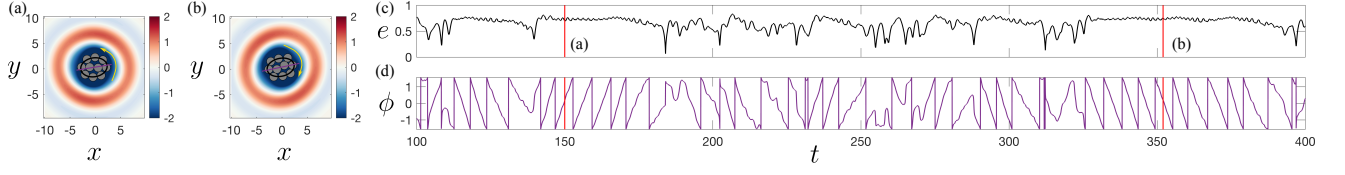

FIG. 3. Intermittent rotating mode of an active wave-particle cluster. A cluster of 10 particles each of size  $a = 1.63$  with  $R = 1.72$  and  $\tau = 4.10$  undergoes chaotic rotation which intermittently changes between (a) counterclockwise and (b) clockwise. Snapshots in (a) and (b) show the particles in gray while their collective wave field is shown in color with peaks in red and troughs in blue (see also Supplemental Video S8). Time series of (c) eccentricity  $e$  and (d) inclination angle  $\phi$  of an ellipse fitted to the center of particle positions. Red lines in panels (c) and (d) correspond to  $t = 150$  and  $t = 352$  at which snapshots of the system are shown in (a) and (b).

types of active particle were to be employed—with one (proton like) type having long-range Coulomb repulsion to augment the short-range repulsion, and the other (neutron like) type only having short-range repulsion—then certain parallels with nuclear physics might become clearer. Adding a third spatial dimension to the model may also be clarifying, in this regard (in adding the third spatial dimension, we would of course no longer have a realistic model for bouncing droplets, but rather would seek in this context an active-particle nuclear analog that is inspired by—but not constrained by—bouncing droplets).

3. It would be interesting to study the *scattering of active-particle clusters from one another*, together with the *scattering of one fast active particle from an active-particle cluster*. Such studies could lead to an analog notion of differential and total scattering cross sections, together with associated concepts such as scattering resonances.
4. Do *active-particle-cluster analogs of nuclear fission and nuclear fusion* exist? If an active-particle-cluster analog of nuclear fission exists, do strongly-deforming collective excitations play a role in the fission mechanism (as least for some of the fission decay channels)?
5. It would be interesting to study a gas of active-

particle clusters, since the average wave barrier surrounding each cluster implies they will repel one another when they touch (unless they collide with sufficiently high speed to initiate a fusion event).

6. Regarding the center-of-mass diffusive motion described in Sec. IV of this Supplemental Material (see, in particular, Fig. 2(c)), it would be interesting to calculate the associated diffusion coefficient as a function of the model parameters  $\tau$ ,  $a$  and  $N$ . One could also determine whether the center-of-mass diffusion is normal or anomalous, i.e., whether or not the variance of the center-of-mass displacement increases linearly with time.
7. Does the center-of-mass of the cluster *recoil* when a particle is ejected? If such a recoil velocity exists, over what timescale is its associated drift erased by the diffusive motion mentioned in item #6 above? Presumably, the time evolution of the probability density for the center-of-mass location, following ejection of a particle from an active-particle cluster, may be modeled using a suitable Fokker-Planck equation [7].
8. Can a *crystal lattice of active-particle clusters* be formed? If such a crystal lattice can indeed be formed, does it exhibit an analog of the Mössbauer effect when one of the active-particle clusters ejects a particle? In particular, when one of the clusters



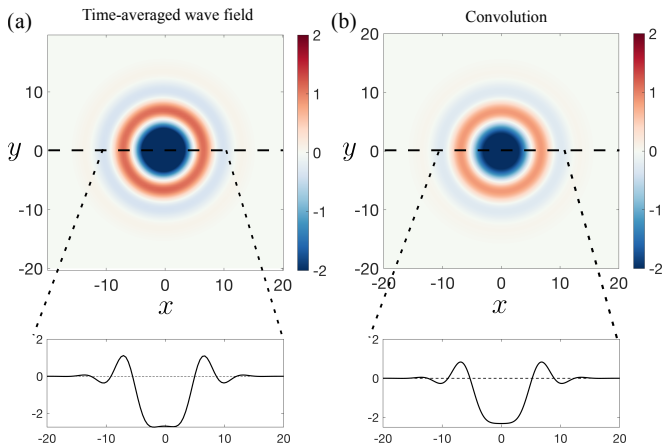

FIG. 4. Comparison of (a) time-averaged wave field (from  $t = 10$  to  $t = 30$ ) from a simulation of a chaotic breathing mode of a cluster of  $N = 10$  particles with particle size  $a = 1.01$ , with (b) the field obtained from convolution of a single-bounce wave field  $W_B(|\mathbf{x}|) = R\tau \cos(|\mathbf{x}|) e^{-\alpha^2|\mathbf{x}|^2}$  for  $N$  particles with a uniform disc whose radius is 3. The radius of the disc is the same extent as the average radius of the region occupied by the particles within the cluster in the simulation. For this simulation, other parameters were fixed to  $\alpha = 0.16$ ,  $R = 0.77$  and  $\tau = 1.09$ .

ejects a particle, does the entire lattice recoil or just the emitting active-particle cluster?

9. The mean particle kinetic energy, relative to the center-of-mass of the active-particle cluster, may be considered as directly proportional to an associated pseudotemperature. Moreover, we may adapt language in the bag-model paper of Chodos *et al.* [8], by likening our active-particle clusters to an active-particle gas bubble that is contained within a “liquid” of approximately constant pressure. Under this view, we can think of the active-particle cluster as being confined via the external pressure that is mentioned in the previous sentence; the cluster radius is then determined by balancing the cluster-expanding force associated with the cluster pseudotemperature, against the cluster-contracting force of the external-“liquid” pressure. In this regard, a key parameter is the active-particle-cluster analog of the “bag constant”, which for our model is given by the mean-field potential per unit area, in the cluster interior (this may be estimated using the convolution integral in Sec. V).
10. How does the pseudotemperature behave in the temporal vicinity of a particle-ejection event? For example, it would be interesting to study whether or not the pseudotemperature increases immediately before an ejection event, and if it has the property analogous to evaporative cooling of becoming reduced after an ejection event.
11. The oscillation frequency associated with our ac-

tive particles is analogous to the Zitterbewegung frequency [9] that naturally occurs in relativistic field theories. Since antiparticles arise inevitably in such theories, *can antiparticle analogs be found in our model?* In particular, does reversing the sign of the waveform  $W$  create an active-particle analog of an antiparticle? If this is indeed the case, then it would be interesting to study analogs of a bound proton-antiproton pair (protonium) or a bound electron-positron pair (positronium) using active-particle pairs that have equal masses but a waveform of opposite sign. Note that in both of these cases we would need to augment the inter-particle force  $F_{ij}^{int}$  with a Coulomb-type term. Can such a model give an analog for particle-antiparticle pair creation and pair annihilation? Alternatively, perhaps a Coulomb term could be used to model particles of opposite charge, with or without the use of a change in sign for  $W$ . Could an analog of a hydrogenic atom be modeled along these lines, using active particles of very different masses together with a Coulomb term corresponding to particles with opposite electric charge? If such a hydrogenic-atom active-particle analog de-excites from a higher-energy state to a lower-energy state, is the resulting energy radiatively carried away in a suitable photon-analog structure that is contained in the wave field?

12. Our governing nonlinear differential equation, namely Eqs. (1) and (2) in the main text, is ultimately derived from a suitable coarse graining of a finite-order underpinning nonlinear differential equation (namely the Navier-Stokes equations of classical fluid mechanics) [1, 10, 11]. Thus the WPEs in our model may be viewed as oscillating soliton-like [12] solutions (breathers [13]) of a governing nonlinear differential equation. This immediately leads to the observation that the key ideas of the present paper might be adapted to study WPEs associated with soliton breather solutions arising from other nonlinear finite-order partial differential equations. Examples include the WPEs known as “oscillons” that arise in periodically driven granular media [14–17], together with the closely related concept of soliton-breather gases [18]. Regarding the former example, it is of relevance in the present context that an early experimental study showed that when such solitonic breather-like states have opposite phase—namely fast-oscillation phases that differ by  $\pi$  radians—the associated structures behave analogously to particle-antiparticle pairs in the sense that “Oscillons of like phase show a short-range repulsive interaction, while oscillons of opposite phase attract and bind” [14]. These remarks are suggestive of a general approach, whereby an underlying finite-order nonlinear partial differential equation which admits breather-like solitons (WPEs) can then lead

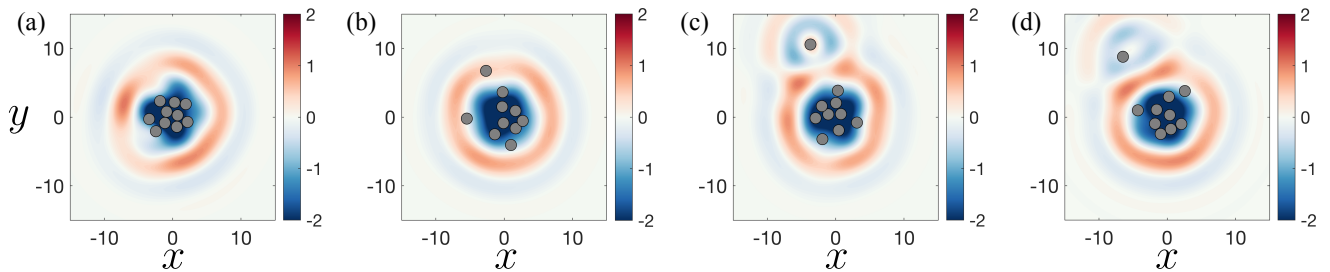

FIG. 5. Decay of an active wave-particle cluster with the ejected particle bound to a “halo” after ejection. A cluster of 10 WPEs of particle size  $a = 1.63$  undergoes chaotic oscillations and ejects a particle which stays bound to the cluster (see also Supplemental Video S9). Snapshots are shown at (a)  $t = 42$ , (b)  $t = 44$ , (c)  $t = 46$  and (d)  $t = 48$ . Other parameters are fixed to  $R = 1.72$ ,  $\alpha = 0.16$  and  $\tau = 7.31$ .

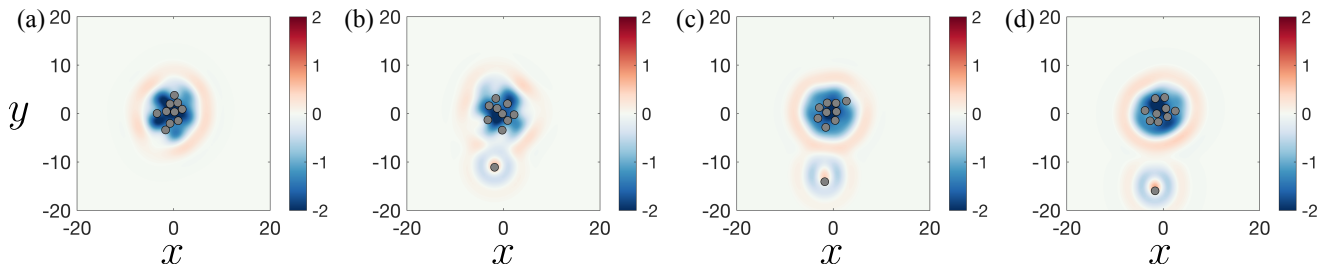

FIG. 6. Decay of an active wave-particle cluster with the particle escaping after ejection. A cluster of 10 WPEs of particle size  $a = 1.63$  undergoes chaotic oscillations and ejects a particle which escapes the cluster (see also Supplemental Video S10). Snapshots are shown at (a)  $t = 26$ , (b)  $t = 28$ , (c)  $t = 30$  and (d)  $t = 32$ . Other parameters are fixed to  $R = 1.72$ ,  $\alpha = 0.23$  and  $\tau = 8.41$ .

to an analog of Eqs. (1) and (2) *for those solitons* (WPEs), namely an emergent integrodifferential equation governing WPE motion. This program is conceptually close to the causal “theory of the Double Solution” due to de Broglie, with what we term the wave form  $W$  being associated with “a continuous  $\Psi$  solution” and what we term the active particle being associated with “another solution ... having an amplitude singularity that is in general mobile” which “would obey a non-linear wave equation” (see pp. 216-218 of the book by de Broglie [19]). Indeed, such a program may be viewed as motivating from whence the “double solution” actually emerges.

We close with some speculations. It is natural to consider a broader context provided by parallels that have been drawn, between classical active wave-particle entities and certain model quantum-mechanical systems [20–22]. In particular, researchers have investigated the possibility that the former, classical, systems may exhibit behaviors (such as entanglement) hitherto thought exclusive to the quantum realm [23, 24]. In a similar vein, ’t Hooft poses the logical possibility that quantum mechanics is a mean-field theory that may emerge—without needing any modification to the existing formalism—via coarse-graining of an as-yet unknown *classical* system such as a suitable cellular-automaton [25]. A key idea, in this regard, is that such underlying classical systems are worth further investigation since they may not be

necessarily ruled out by standard “no go” arguments associated with Bell inequalities and hidden-variable theories [25]. While we are unable at this stage to substantiate any claim regarding the applicability of our findings to the genuinely quantum-mechanical domain of nuclear and composite-particle physics, it is nevertheless interesting to further explore the extent to which other nuclear-physics and composite-particle phenomena may have direct analogs with entirely-classical clusters of wave-particle entities. In pursuing such a line of inquiry, it appears likely that a different form for the wave form  $W$  may need to be employed. *Can a suitably modified form of the classical integrodifferential expressions in Eqs. (1) and (2) of the main text, with a suitably modified wave form and a suitably modified repulsive term, be amenable to coarse graining which subsequently leads to a formalism that more closely approximates an emergent quantum system? Can the integrodifferential equation itself be obtained via breathing-mode solitonic solutions to an underpinning finite-order partial differential equation?*

## SUPPLEMENTAL VIDEOS

**Supplemental Video S1:** Video of the breathing mode of the active wave-particle cluster corresponding to Fig. 2(a) in the main text.

**Supplemental Video S2:** Video of the crushing mode of the active wave-particle cluster corresponding

to Fig. 2(b) in the main text.

**Supplemental Video S3:** Video of the rotating mode of the active wave-particle cluster corresponding to Fig. 2(c) in the main text.

**Supplemental Video S4:** Video of the vibration mode of the active wave-particle cluster corresponding to Fig. 2(d) in the main text.

**Supplemental Video S5:** Video of the compression mode of the active wave-particle cluster corresponding to Fig. 2(e) in the main text.

**Supplemental Video S6:** Video of the rotating mode of the active wave-particle cluster corresponding to Fig. 2(f) in the main text.

**Supplemental Video S7:** Video of the chaotic breath-

ing mode of the active wave-particle cluster corresponding to Fig. 2 in the Supplemental Material.

**Supplemental Video S8:** Video of the intermittent rotating mode of the active wave-particle cluster corresponding to Fig. 3 in the Supplemental Material.

**Supplemental Video S9:** Video showing decay of an active wave-particle cluster with bounded “halo” particle after ejection corresponding to Fig. 5 in the Supplemental Material.

**Supplemental Video S10:** Video showing decay of an active wave-particle cluster with escaping particle after ejection corresponding to Fig. 6 in the Supplemental Material.

- 
- [1] A. U. Oza, R. R. Rosales, and J. W. M. Bush, *J. Fluid Mech.* **737**, 552 (2013).
  - [2] R. N. Valani, A. C. Slim, and T. Simula, *Phys. Rev. Lett.* **123**, 024503 (2019).
  - [3] N. B. Padhan and R. Pandit, *Phys. Rev. Res.* **5**, L032013 (2023).
  - [4] M. Durey, P. A. Milewski, and J. W. M. Bush, *Chaos* **28**, 096108 (2018).
  - [5] Y. Ye, X. Yang, H. Sakurai, and B. Hu, *Nat. Rev. Phys.* **7**, 21 (2025).
  - [6] K. S. Krane, *Introductory Nuclear Physics* (Wiley, 1987).
  - [7] H. Risken, *The Fokker-Planck Equation*, 2nd ed. (Springer Verlag, Berlin, 1989).
  - [8] A. Chodos, R. L. Jaffe, K. Johnson, C. B. Thorn, and V. F. Weisskopf, *Phys. Rev. D* **9**, 3471 (1974).
  - [9] J. J. Sakurai, *Advanced Quantum Mechanics* (Addison-Wesley, 1967).
  - [10] J. Moláček and J. W. M. Bush, *J. Fluid Mech.* **727**, 582 (2013).
  - [11] J. Moláček and J. W. M. Bush, *J. Fluid Mech.* **727**, 612 (2013).
  - [12] Y. S. Kivshar and G. P. Agrawal, *Optical Solitons: From Fibers to Photonic Crystals* (Academic Press, 2003).
  - [13] N. Akhmediev, J. M. Soto-Crespo, and G. Town, *Phys. Rev. E* **63**, 056602 (2001).
  - [14] P. B. Umbanhowar, F. Melo, and H. L. Swinney, *Nature* **382**, 793 (1996).
  - [15] E. Clément, L. Vanel, J. Rajchenbach, and J. Duran, *Phys. Rev. E* **53**, 2972 (1996).
  - [16] L. S. Tsimring and I. S. Aranson, *Phys. Rev. Lett.* **79**, 213 (1997).
  - [17] I. S. Aranson and L. S. Tsimring, *Rev. Mod. Phys.* **78**, 641 (2006).
  - [18] G. El and A. Tovbis, *Phys. Rev. E* **101**, 052207 (2020).
  - [19] L. de Broglie, *Non-Linear Wave Mechanics: A Causal Interpretation* (Elsevier, 1960).
  - [20] J. W. M. Bush, *Annu. Rev. Fluid Mech.* **47**, 269 (2015).
  - [21] J. W. M. Bush and A. U. Oza, *Rep. Prog. Phys.* **84**, 017001 (2020).
  - [22] J. W. M. Bush, K. Papatryfonos, and V. Frumkin, “The state of play in hydrodynamic quantum analogs,” in *Advances in Pilot Wave Theory: From Experiments to Foundations*, edited by P. Castro, J. W. M. Bush, and J. Croca (Springer International Publishing, Cham, 2024) pp. 7–34.
  - [23] R. N. Valani, A. C. Slim, and T. Simula, *Chaos* **28**, 096104 (2018).
  - [24] K. Papatryfonos, L. Vervoort, A. Nachbin, M. Labousse, and J. W. M. Bush, *Phys. Rev. Fluids* **9**, 084001 (2024).
  - [25] G. ’t Hooft, *The Cellular Automaton Interpretation of Quantum Mechanics* (Springer, Cham, 2016).
